# Supplementary material for: Nonlinear Bias of Cosmological Halo Formation in the Early Universe
Source: arXiv:1407.2637 source file (2015-04-01)
Supplement: Supplementary file 1 [file supplement.pdf]

Mon. Not. R. Astron. Soc. **000**, 000–000 (0000) Printed 6 March 2015 (MN LaTeX style file v2.2)

# Supplementary Material: Nonlinear Bias of Cosmological Halo Formation

Kyungjin Ahn,[1⋆] Ilian T. Iliev,[2] Paul R. Shapiro[3] and Chaichalit B. Srisawat[2]
[1] *Department of Earth Sciences, Chosun University, Gwangju 501-759, Korea*
[2] *Astronomy Centre, Department of Physics and Astronomy, Pevensey II Building, University of Sussex, Falmer, Brighton BN1 9QH*
[3] *Department of Astronomy, University of Texas, Austin, TX 78712-1083, USA*

6 March 2015

**ABSTRACT**
We provide supplementary material, composed of 14 figures relevant to the main manuscript of the paper, "Nonlinear Bias of Cosmological Halo Formation". Some of these figures are cross-referenced in the main paper.

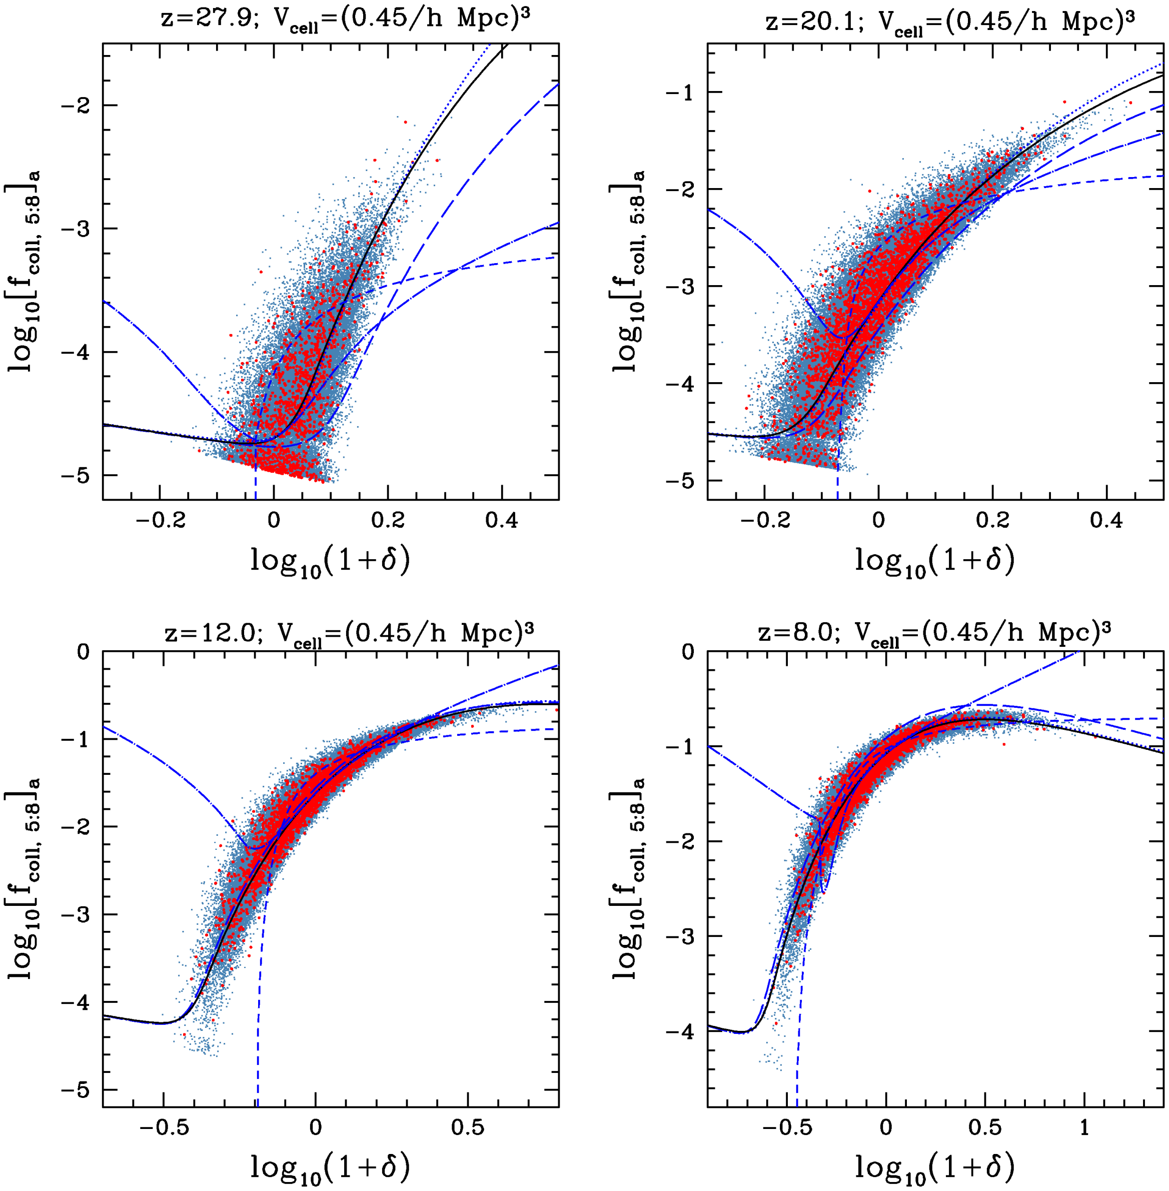


**Figure 1.** Correlation between the fraction of mass collapsed into minihaloes ($f_{\rm coll,\,5:8}$) and the cell overdensity $\delta$ in the 6.3/h Mpc box, where the box is sampled by $14^3$ grid-cells. Conventions for plotting follow those of Fig. 2 of the main paper.

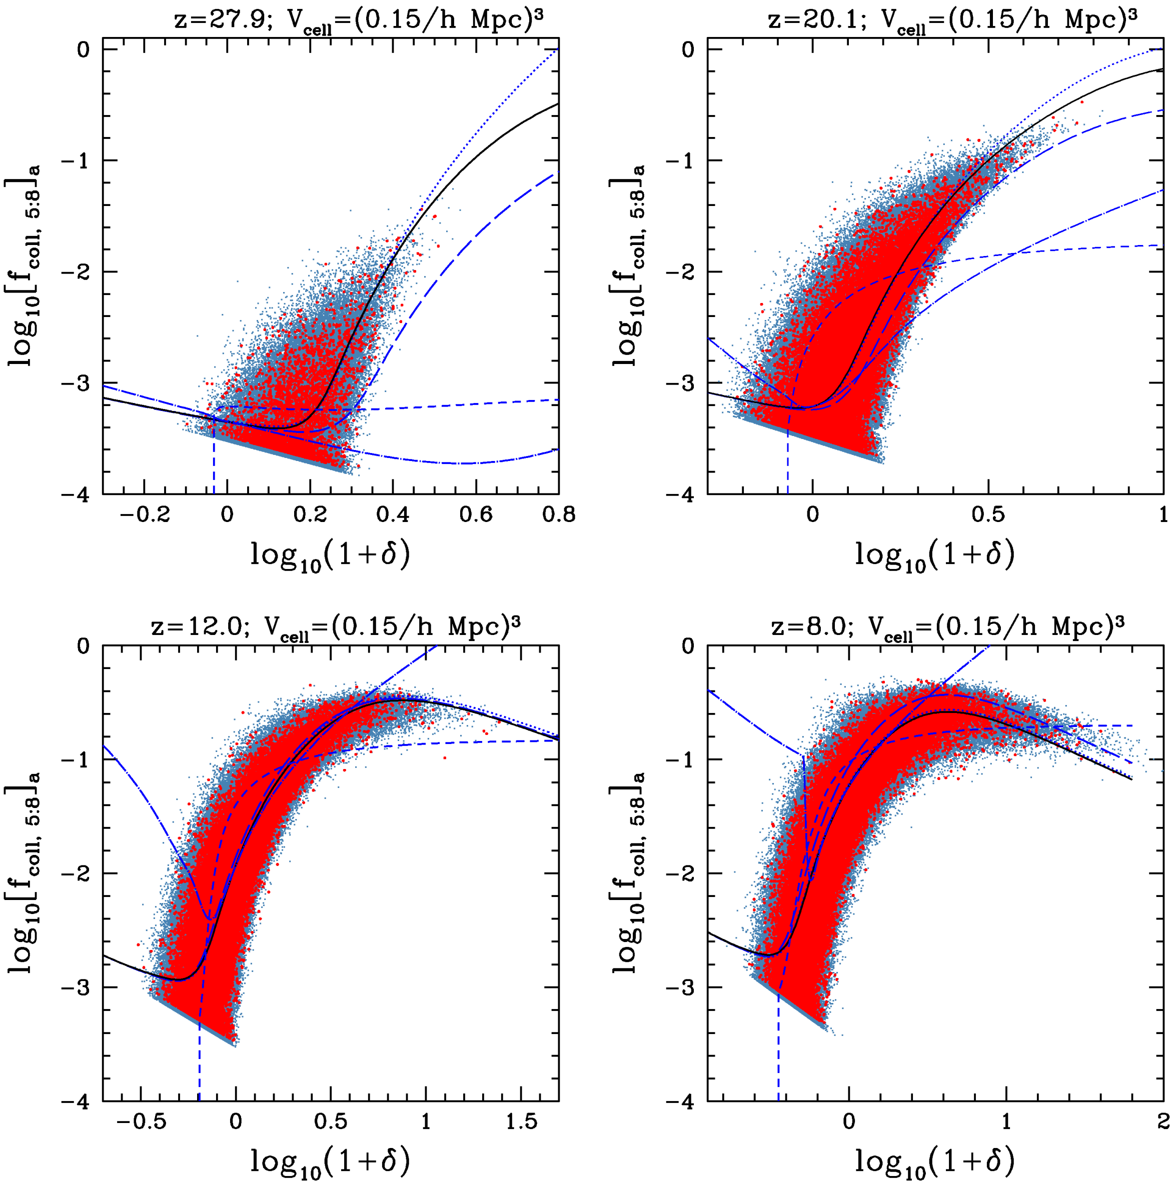


**Figure 2.** Correlation between the fraction of mass collapsed into minihaloes ($f_{\rm coll,\,5:8}$) and the cell overdensity $\delta$ in the 6.3/h Mpc box and 20/h Mpc box, sampled by $44^3$ and $135^3$ cells, respectively. Conventions for plotting follow those of Fig. 2 of the main paper.

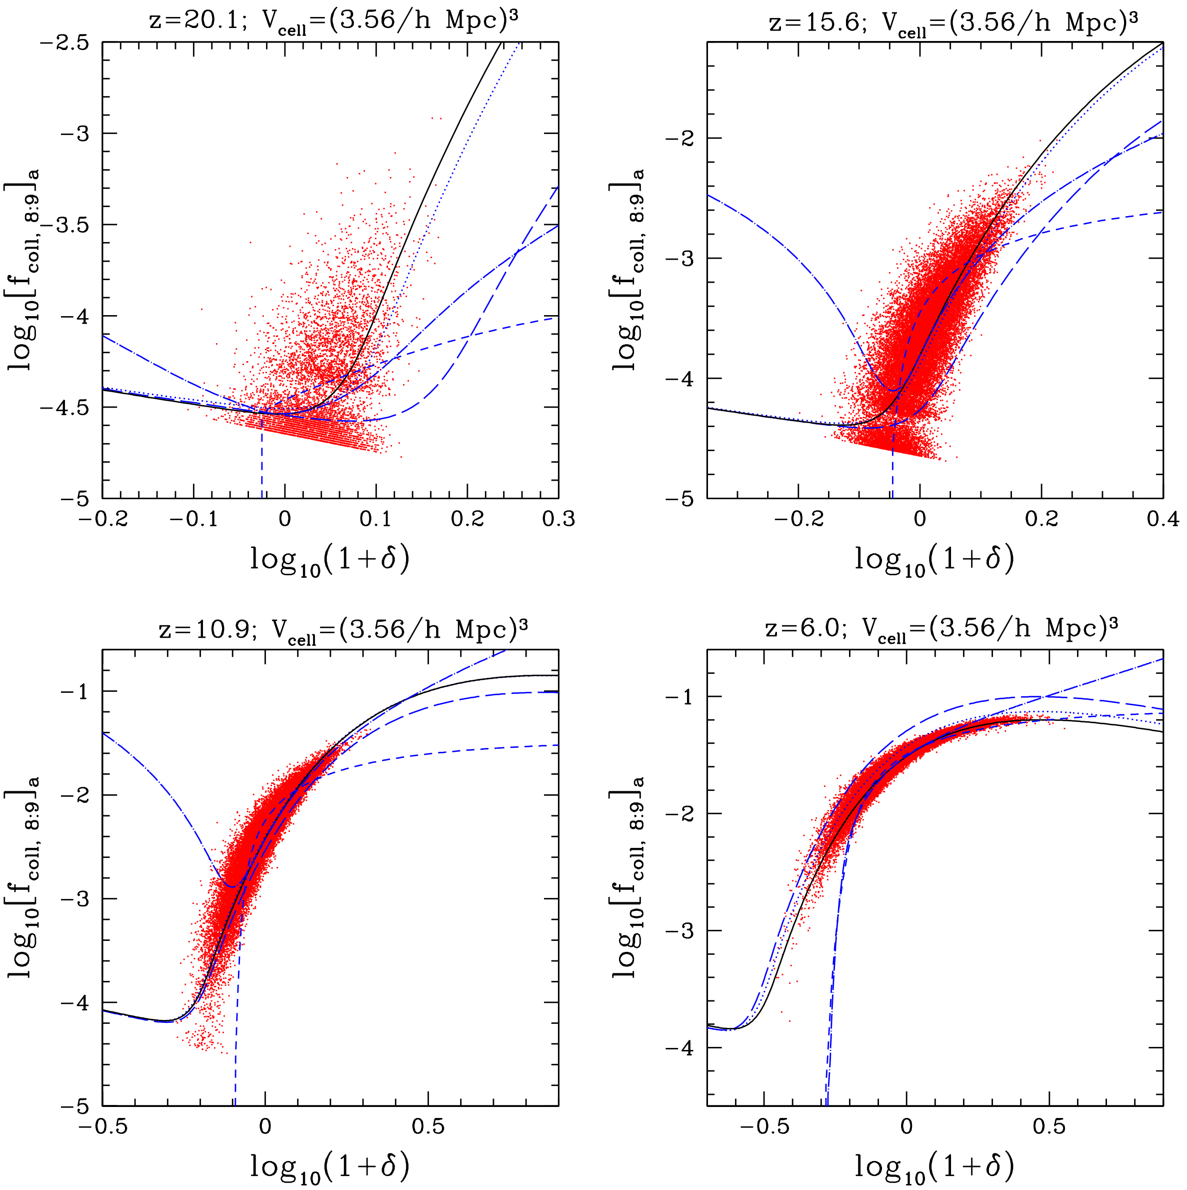


**Figure 3.** Correlation between the fraction of mass collapsed ($f_{\rm coll,\,8:9}$) into LMACHs ($M = 10^8 - 10^9\,M_\odot$) and the cell overdensity $\delta$ in the 114/h Mpc box, where the box is sampled by $32^3$ grid-cells. Conventions for plotting follow those of Fig. 2 of the main paper, except for the data points (red point).

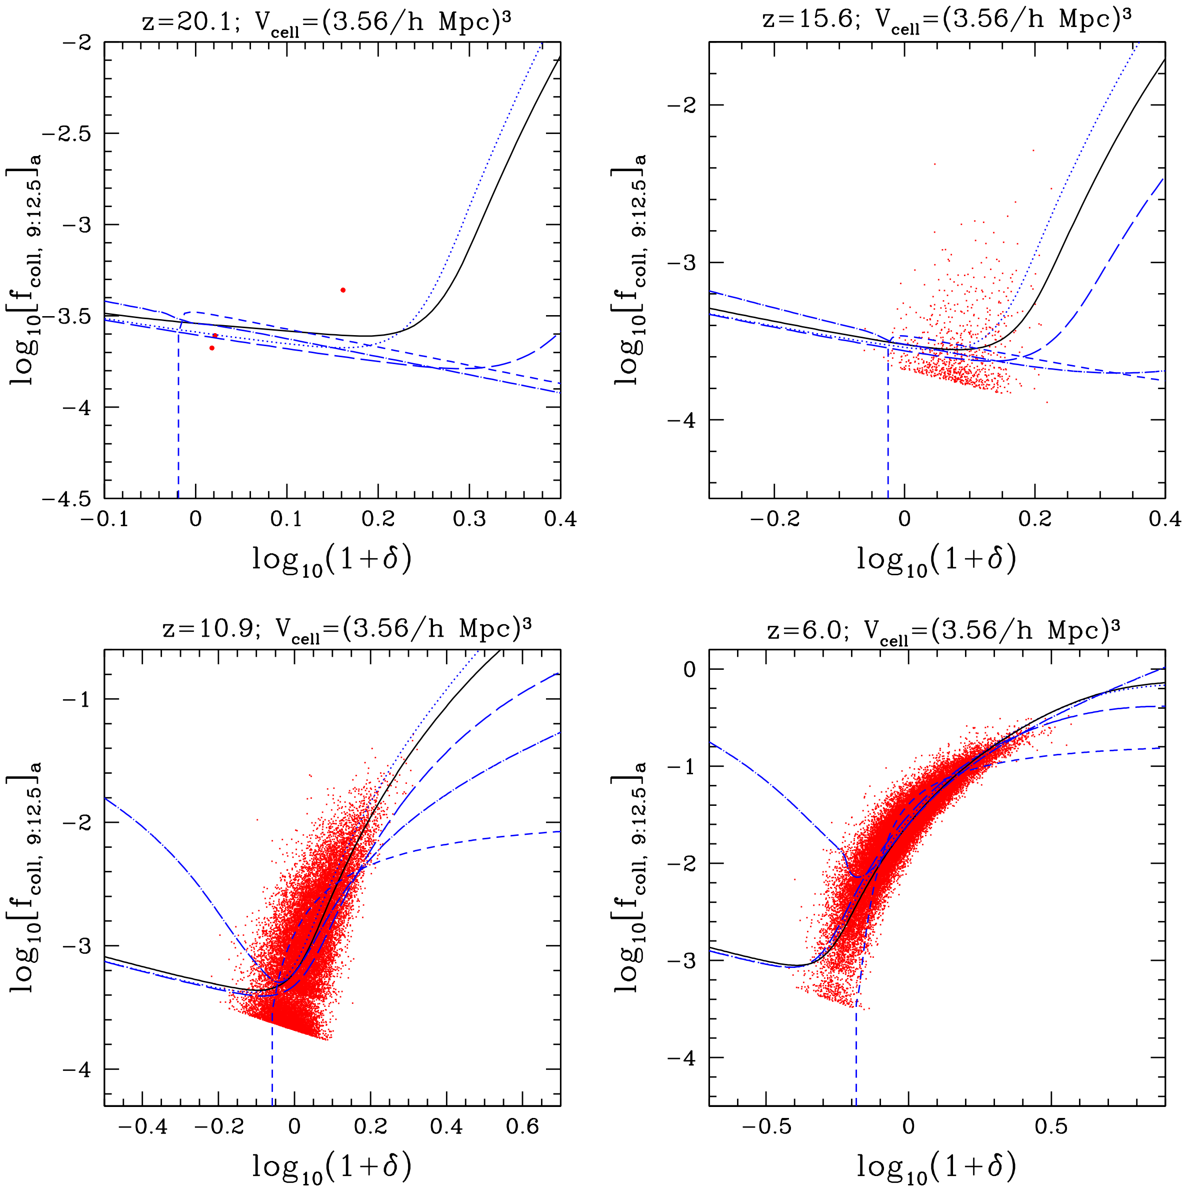


**Figure 4.** Correlation between the fraction of mass collapsed ($f_{\mathrm{coll},\,9:12.5}$) into HMACHs ($M = 10^9 - 10^{12.5}\,M_\odot$, where the maximum mass is roughly the mass of a cell) and the cell overdensity $\delta$ in the 114/h Mpc box, where the box is sampled by $32^3$ grid-cells. Conventions for plotting follow those of Fig. 2 of the main paper, except for the data points (red point).

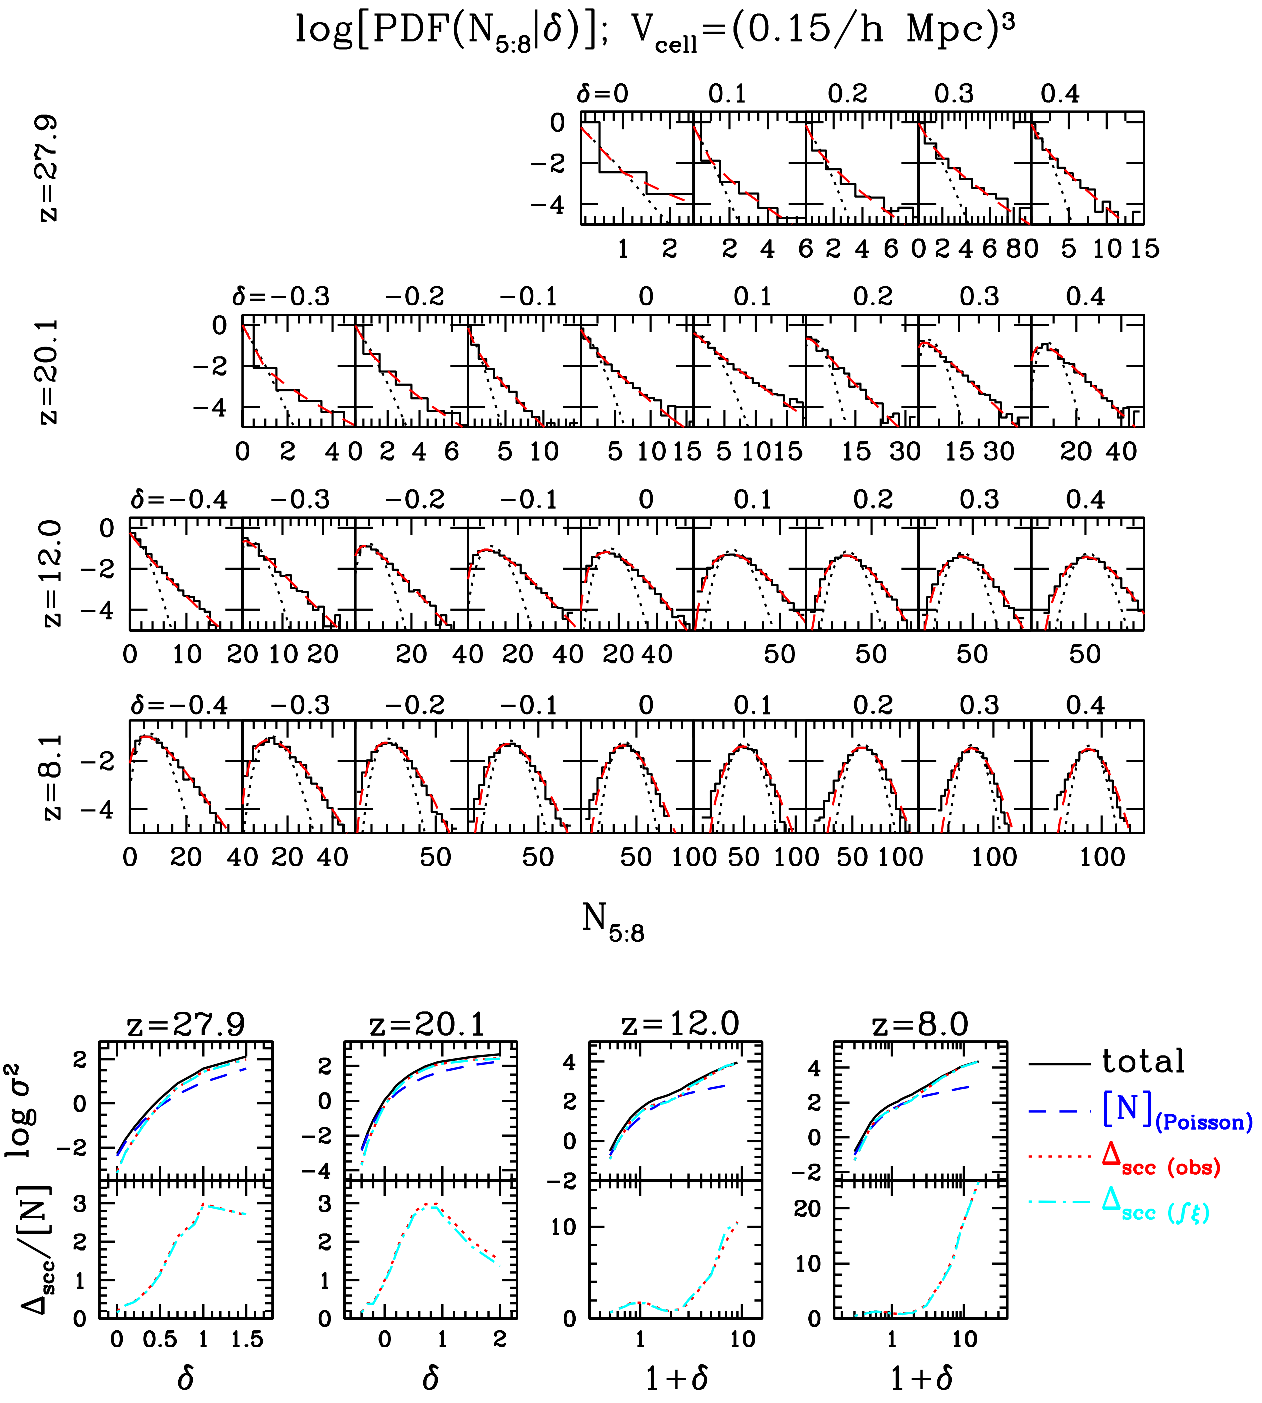


**Figure 5.** (A) Same as Fig. 6(A) of the main paper, but of cells with Eulerian volume $(0.15/h\,\mathrm{Mpc})^3$ in 20/h Mpc box. (B) Same as Fig. 6(B) of the main paper. Here we also find that $\Delta_{\rm scc} > 0$ with this cell size at any $\delta$ at $z \leqslant 28$. Note the hugely nonlinear regime of $\delta$ observed at $z \leqslant 12$.

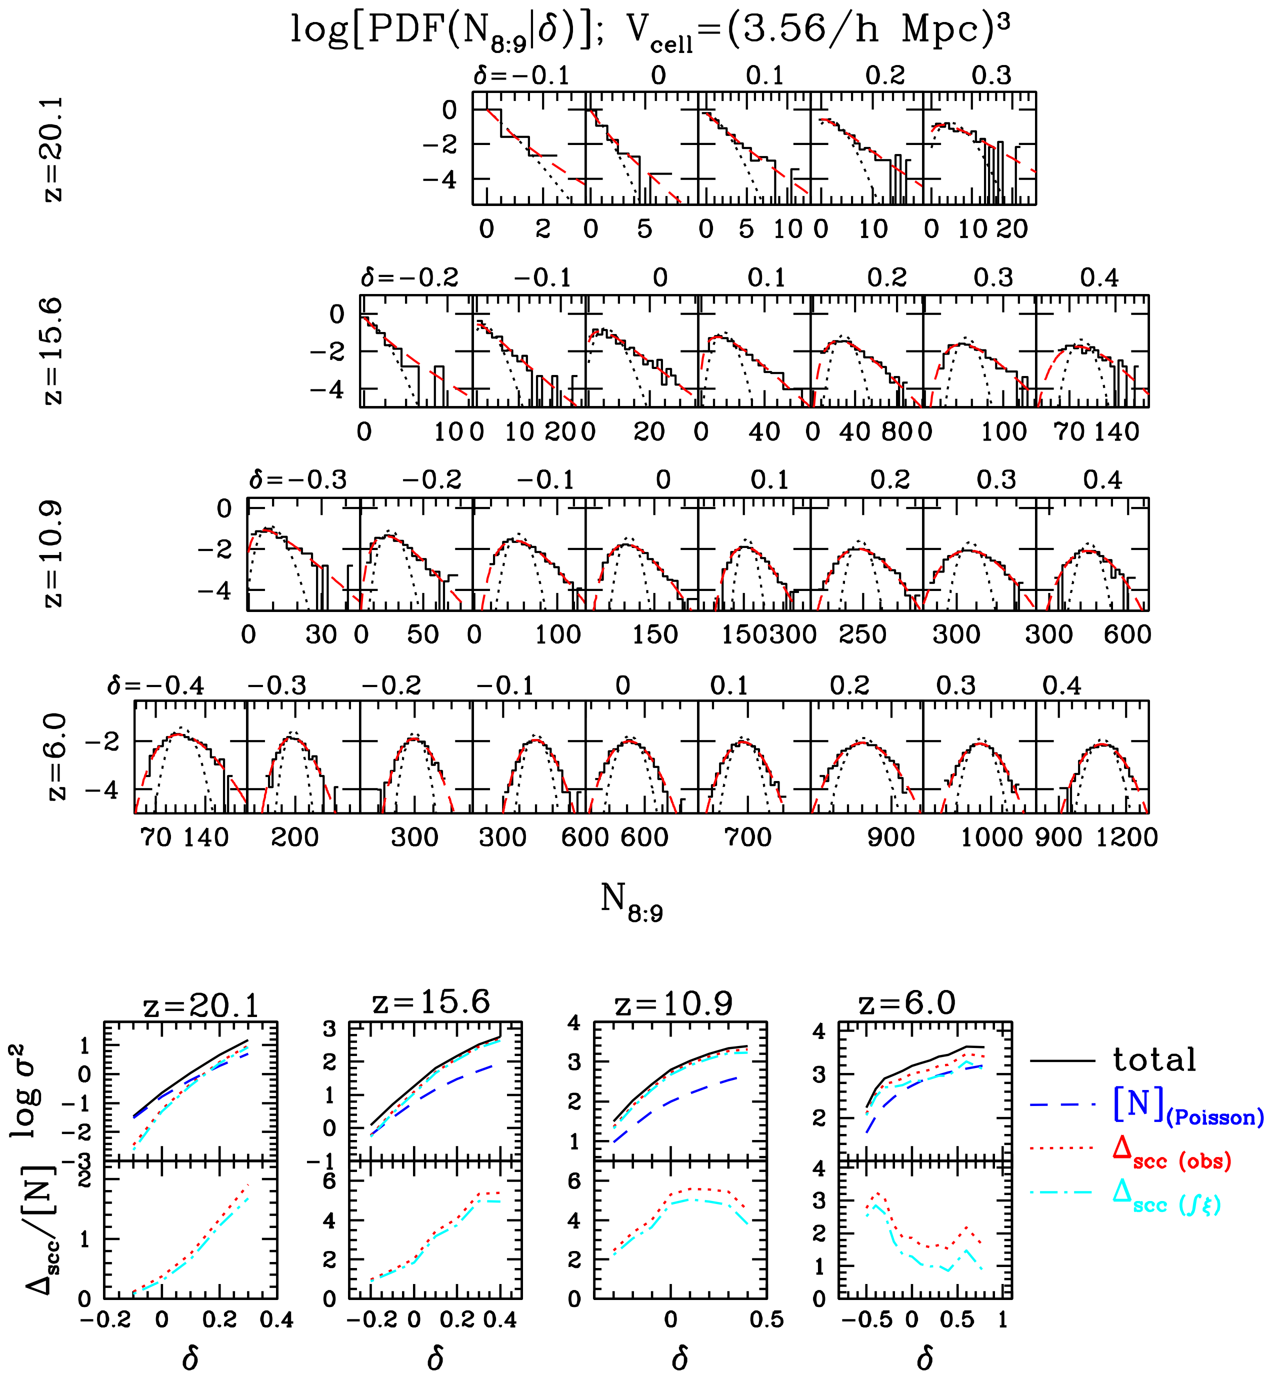


**Figure 6.** (A) PDFs of LMACHs at given overdensity $\delta$ in cells with Eulerian volume $(3.56/h\,\mathrm{Mpc})^3$ in $114/h$ Mpc box. (B) Same as Fig. 6(B) of the main paper. Here we also find that $\Delta_{\rm scc} > 0$ with this cell size at any $\delta$ at $z \leqslant 20$.

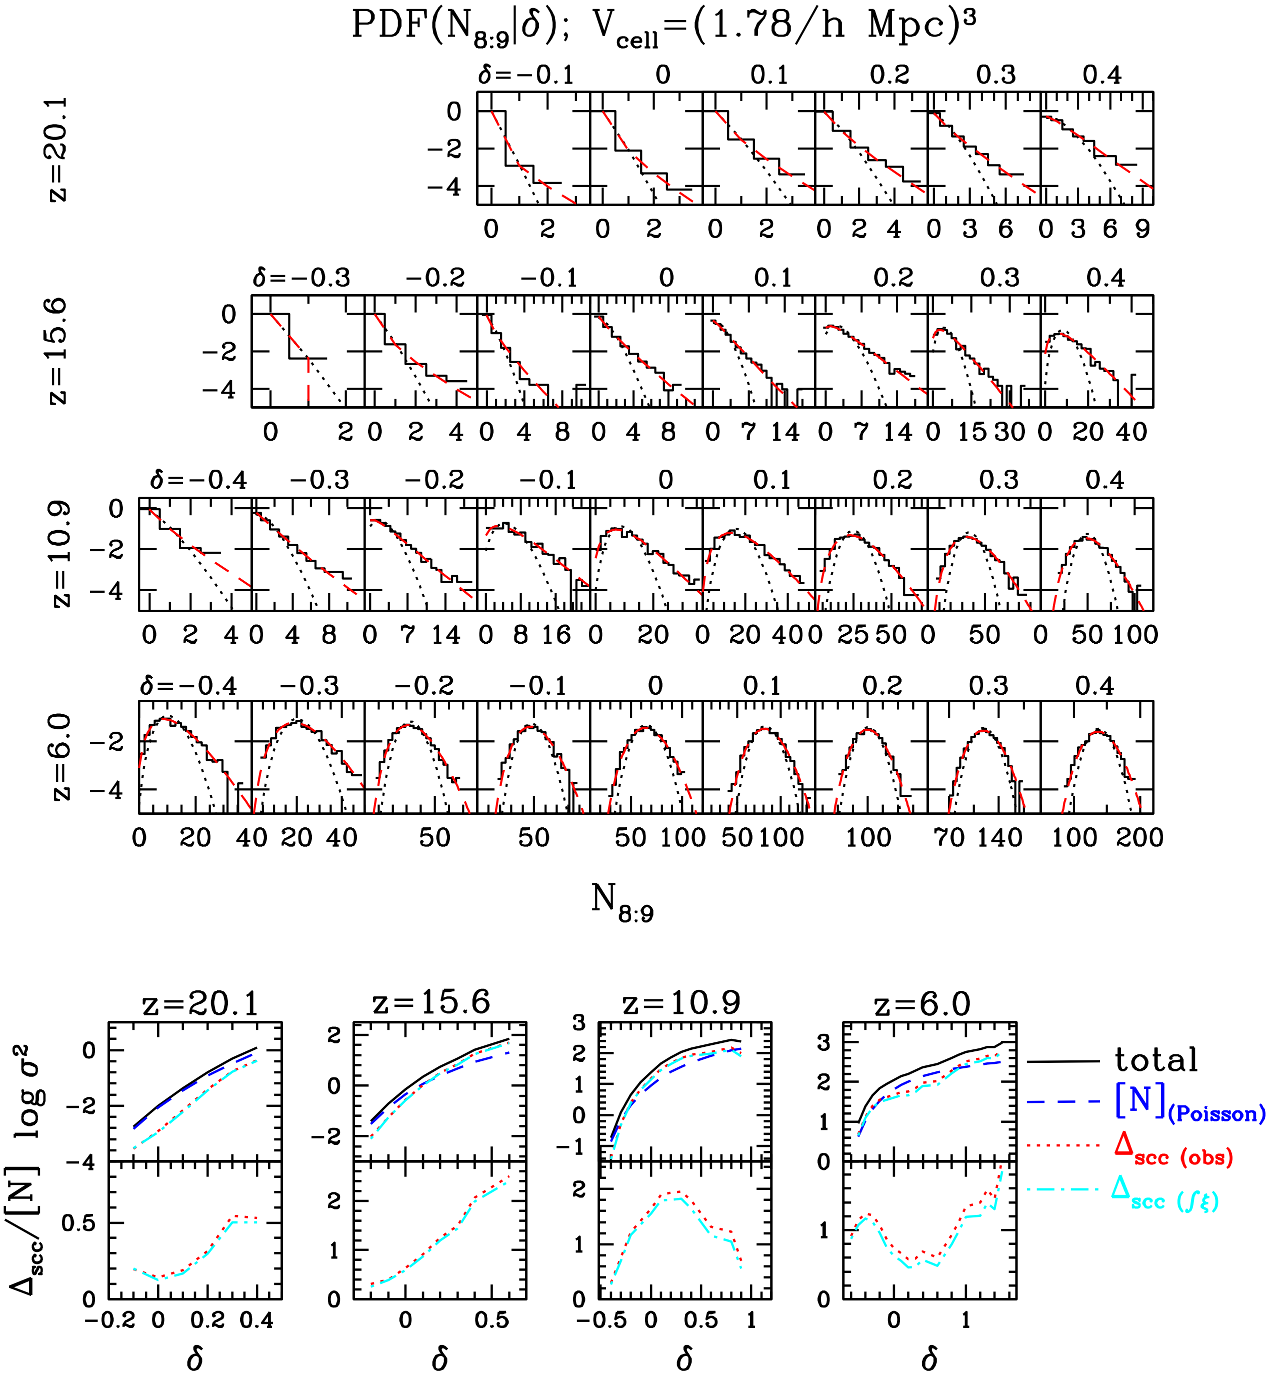


**Figure 7.** (A) PDFs of LMACHs at given overdensity $\delta$ in cells with Eulerian volume $(1.78/h\,\mathrm{Mpc})^3$ in $114/h$ Mpc box. (B) Same as Fig. 6(B) of the main paper. Here we also find that $\Delta_{\rm scc} > 0$ with this cell size at any $\delta$ at $z \leqslant 20$.

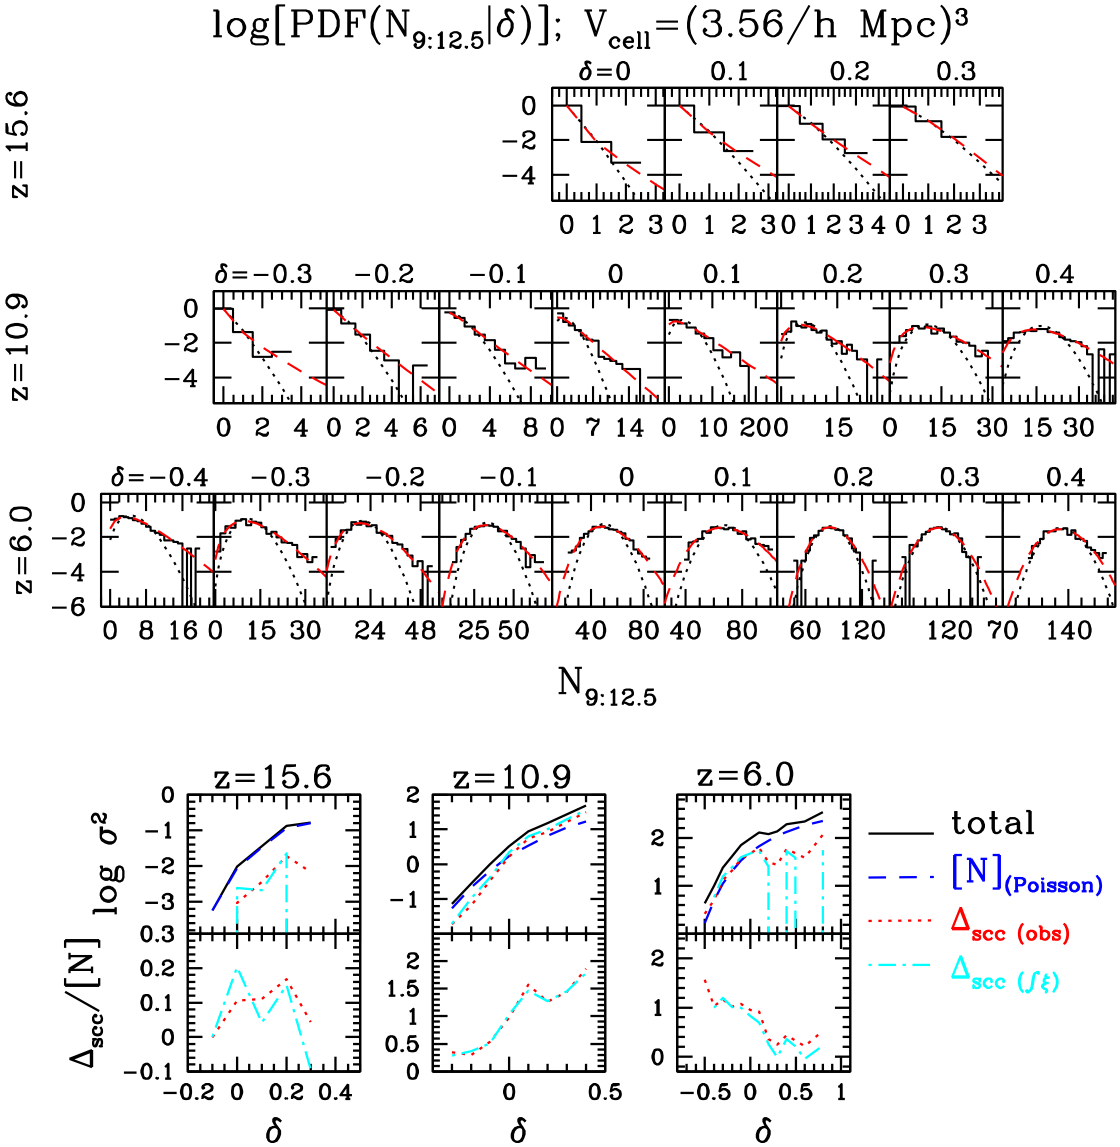


**Figure 8.** (A) PDFs of HMACHs at given overdensity $\delta$ in cells with Eulerian volume $(3.56/h\,\mathrm{Mpc})^3$ in $114/h$ Mpc box. (B) Same as Fig. 6(B) of the main paper. Here we also find that $\Delta_{\rm scc} > 0$ with this cell size at any $\delta$ at $z \leqslant 16$ except at $\delta = -0.1$ at $z = 15.6$ where $\Delta_{\rm scc} = 0$. Overall, at $z = 15.6$, PDFs of HMACHs at any $\delta$ may be approximated well by pure Poisson distribution, as the ratio $\Delta_{\rm scc}/\,[N]$ is small.

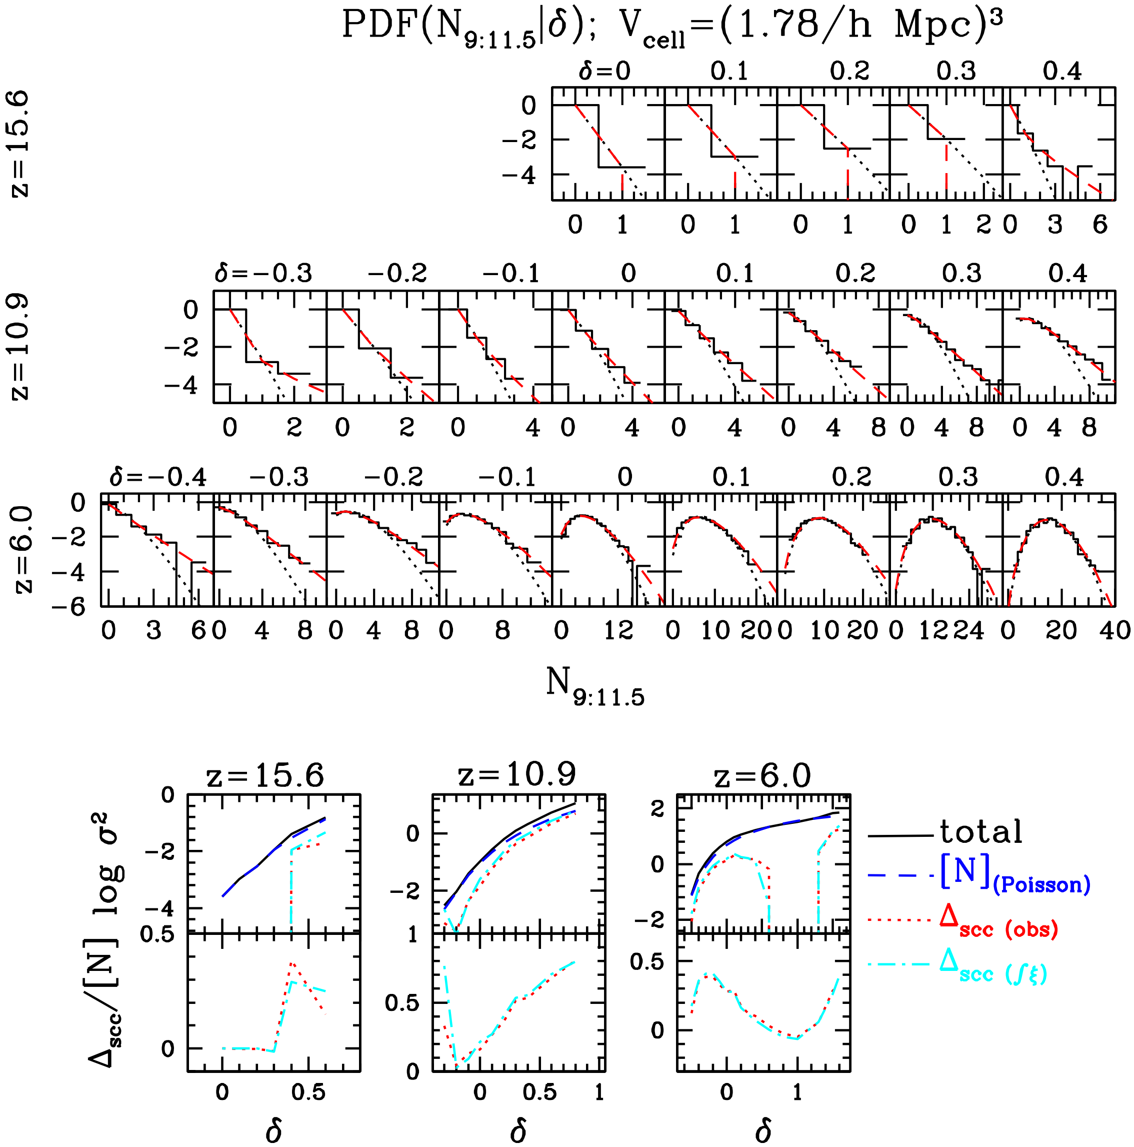


**Figure 9.** (A) PDFs of HMACHs at given overdensity $\delta$ in cells with Eulerian volume $(1.78/h\,\mathrm{Mpc})^3$ in $114/h$ Mpc box. (B) Same as Fig. 6(B) of the main paper. The outliers compared to pure Poisson distribution is overall small, albeit $\Delta_{\rm scc}$ is comparable to $[N]$ at $\delta \gtrsim 0.5$. In some cases $\Delta_{\rm scc} < 0$, which may be an indication of overall anti-correlation in the sub-cell scale such that $\xi_{12} < 0$ (see equation 19 of the main paper): however, the ratio is too small to draw a firms conclusion. Overall, PDFs of HMACHs may be approximated reasonably well by pure Poisson distribution in the redshift range $6 \lesssim z \lesssim 15$ and the range of $\delta \lesssim 0.5$.

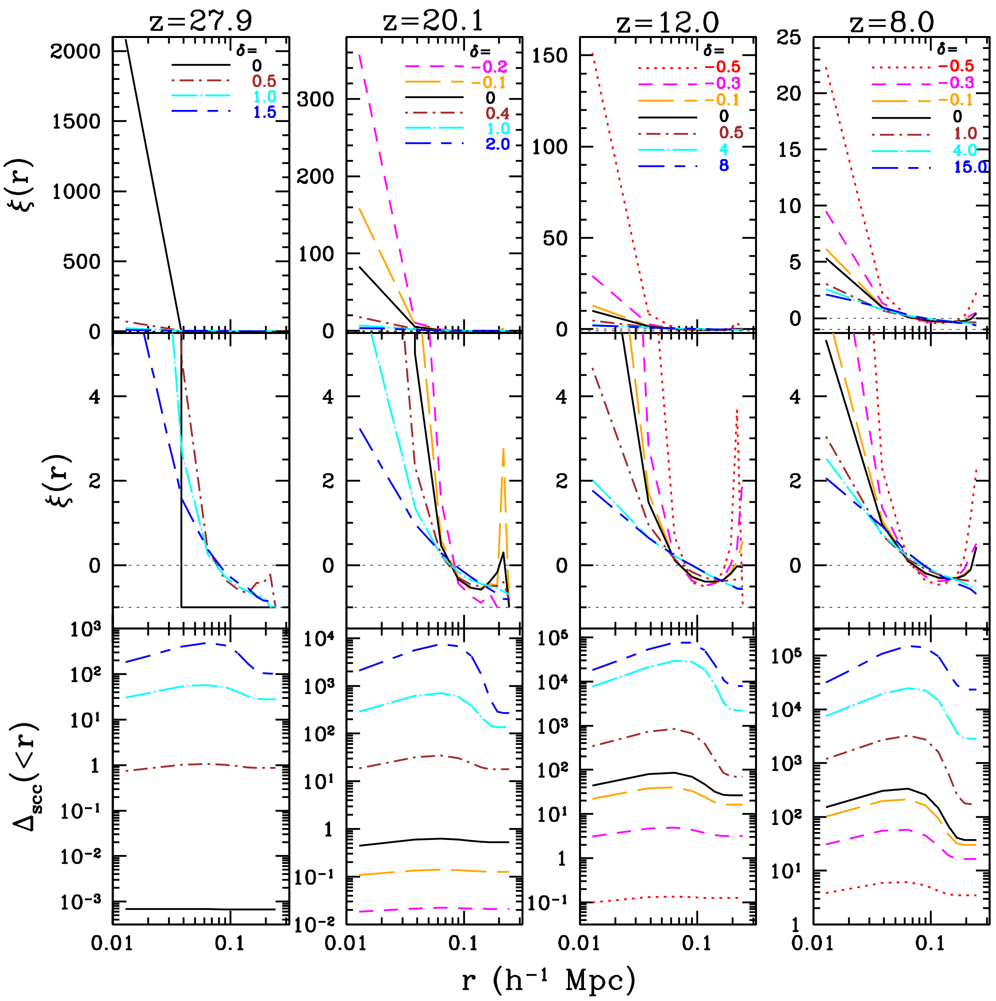


**Figure 10.** Sames as fig 7 of the main paper but with $V_{\rm cell} = (0.15/h)^3$ Mpc.

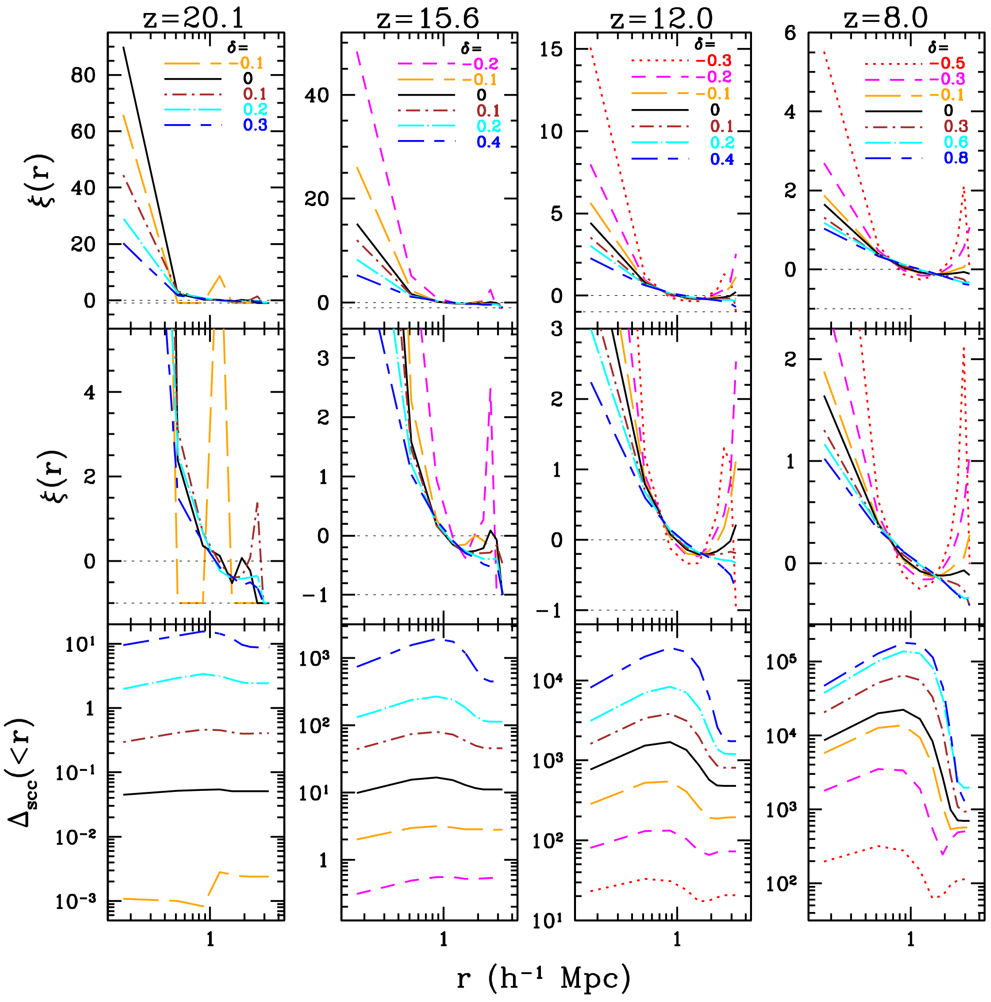


**Figure 11.** Same as fig 7 of the main paper but for LMACHs inside $114/h$ Mpc box with $V_{\rm cell} = (3.56/h)^3$ Mpc.

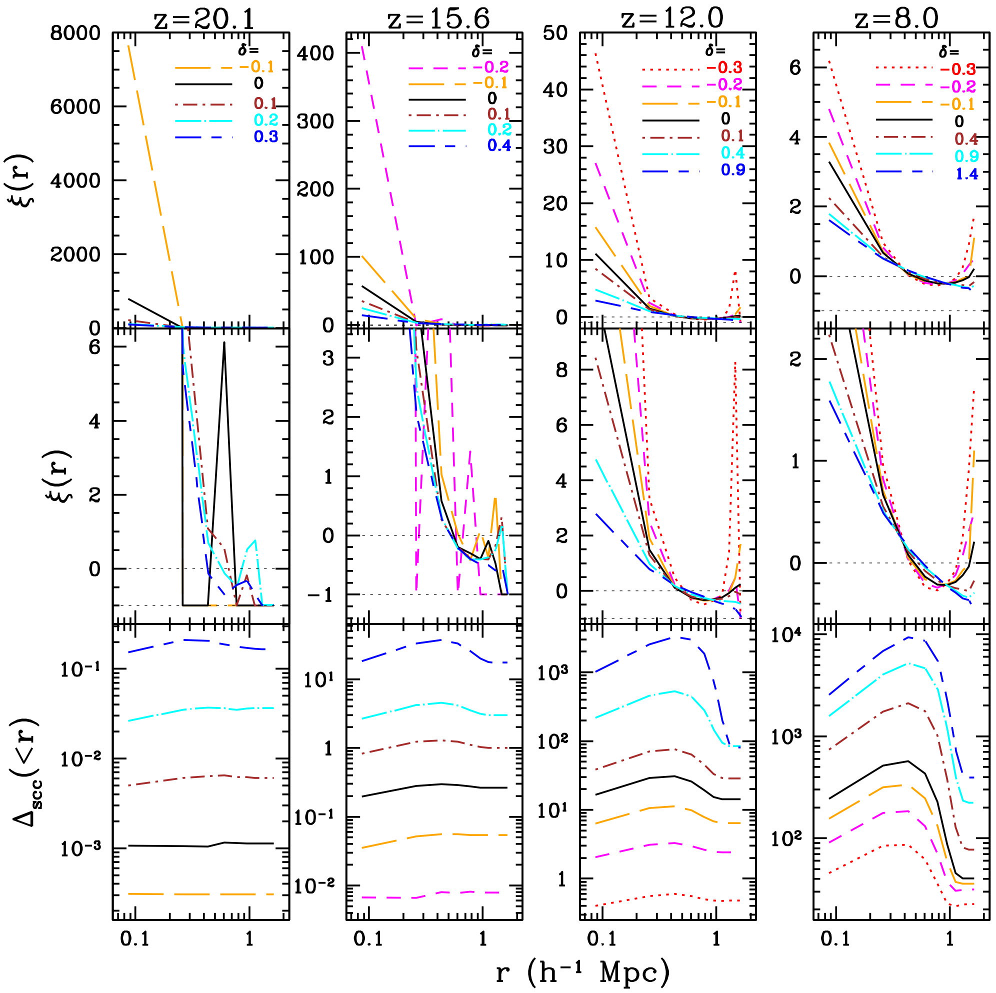


**Figure 12.** Same as fig 11 but with $V_{\rm cell} = (3.56/h)^3\,$Mpc.

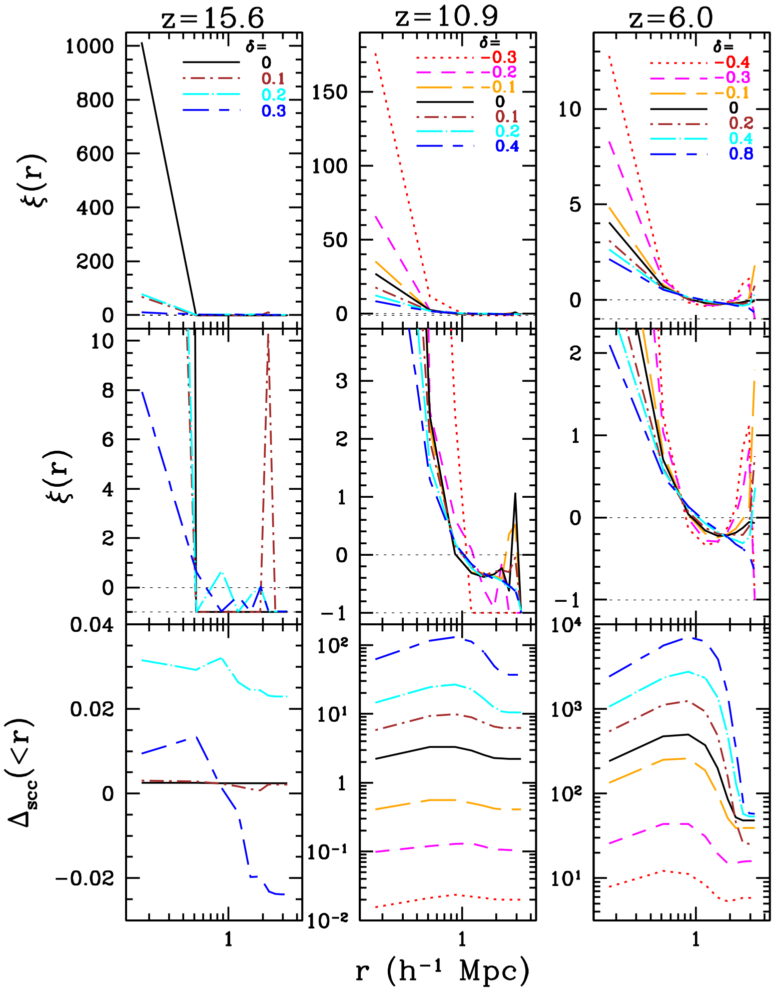


**Figure 13.** Same as Fig. 7 of the main paper but for HMACHs inside $114/h$ Mpc box with $V_{\rm cell} = (3.56/h)^3$ Mpc.

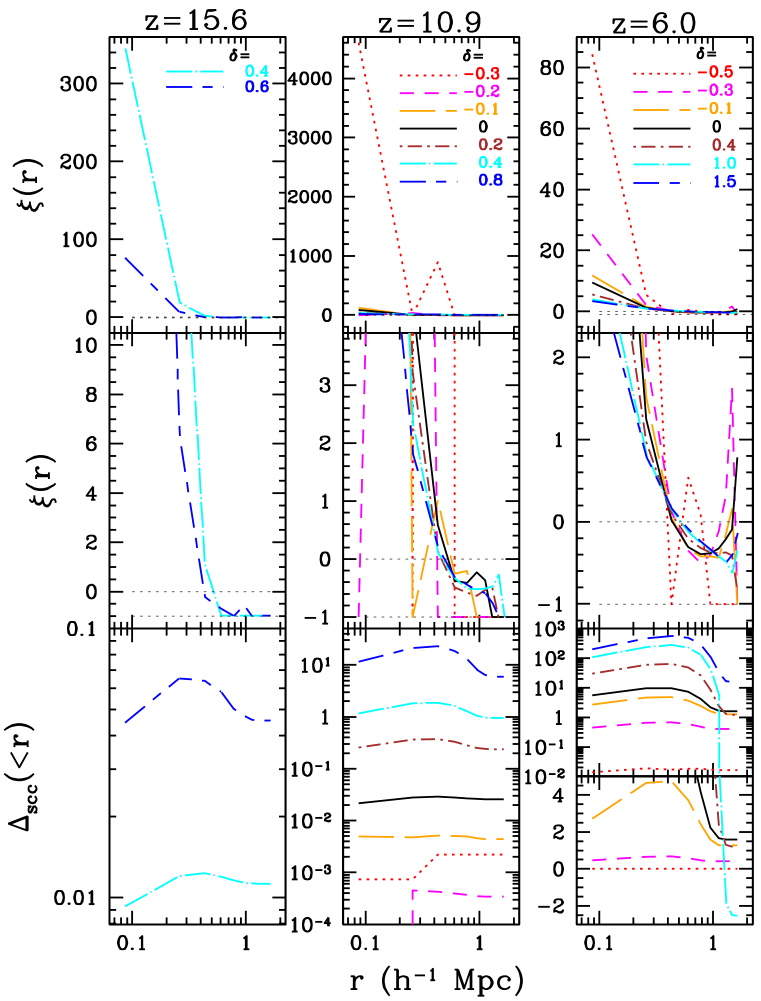


**Figure 14.** Same as fig 13 but with $V_{\rm cell} = (1.78/h)^3$ Mpc.
